# Supplementary material for: Astrophysical Objects in Modified Theories of Gravity
Source: arXiv:2605.21564 source file (2026-05-23)
Supplement: Supplementary file 2 [file AppendixTemplate.tex]

% Appendix Template

\chapter{Appendix Title Here} % Main appendix title

\label{AppendixX} % Change X to a consecutive letter; for referencing this appendix elsewhere, use \ref{AppendixX}

\lhead{Appendix X. \emph{Appendix Title Here}} % Change X to a consecutive letter; this is for the header on each page - perhaps a shortened title

Write your Appendix content here.
